# Supplementary material for: LucidDreaming: Controllable Object-Centric 3D Generation
Source: arXiv:2312.00588 source file (2024-08-09)
Supplement: Supplementary file 1 [file supp.tex]

\clearpage
\setcounter{page}{1}
\maketitlesupplementary
\appendix
\input{supp/Overview}
\input{supp/Tech}
\input{supp/Dataset}
\input{supp/Visualization}
\input{supp/Discussion}
% \clearpage

\begin{figure*}[!]
   \centering
   \vspace{5.0cm}
    \includegraphics[width=1.0\linewidth]{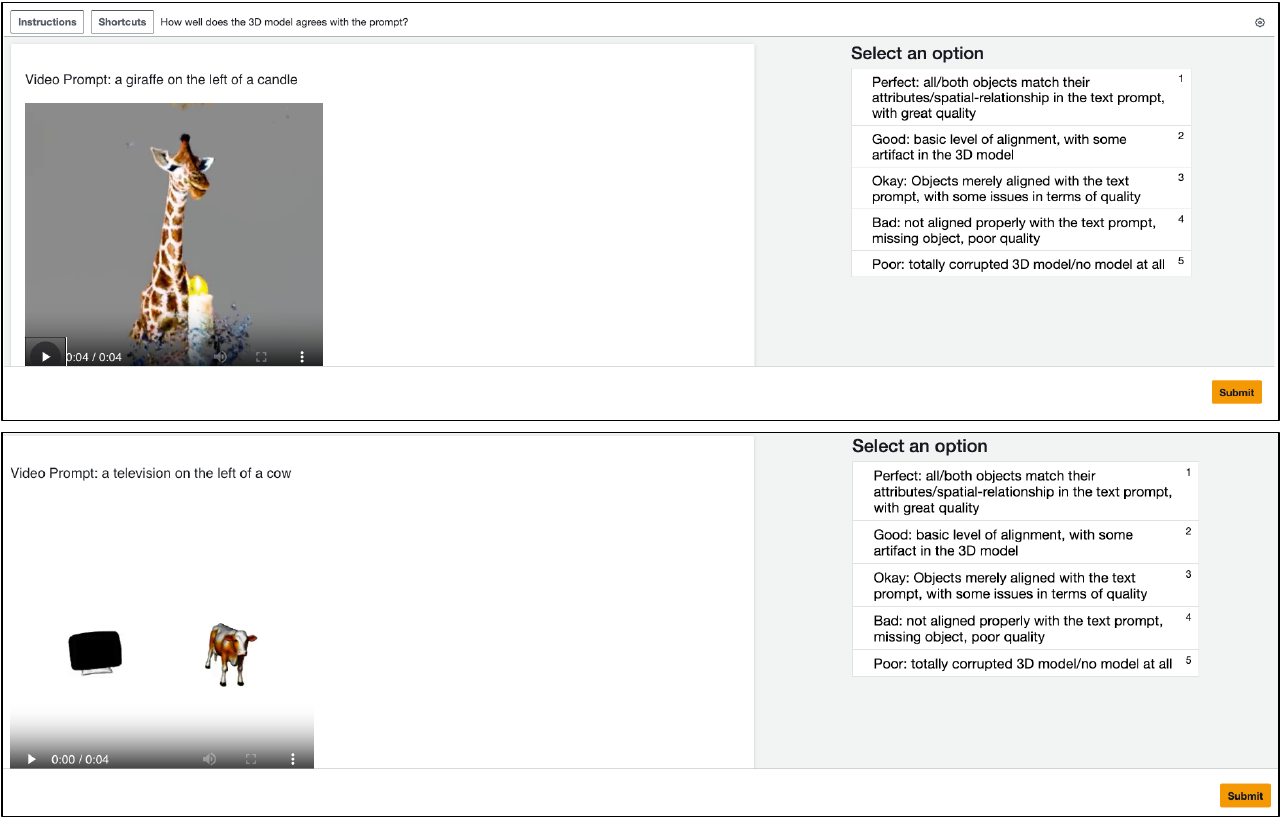}
    \caption{Visualization of Amazon Mechanical Turk (AMT) for Human Annotations.}
    \label{fig:vis_amt}
\end{figure*}

\begin{figure*}[!]
   \centering
    \includegraphics[width=1\linewidth]{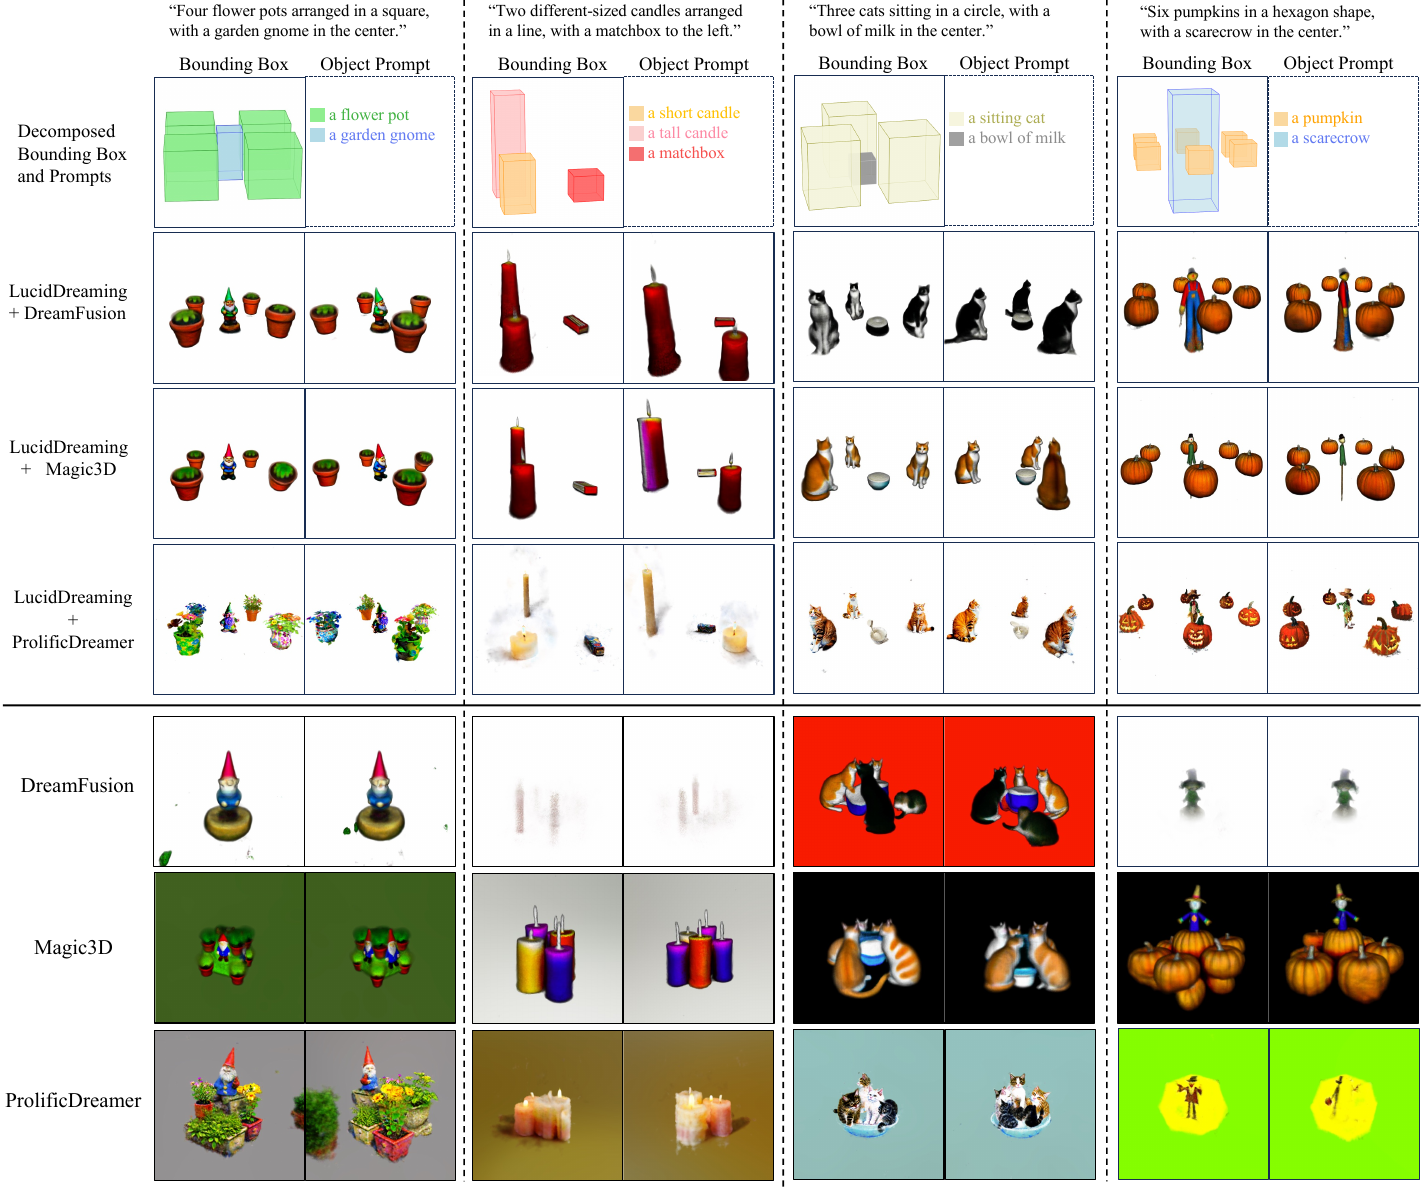}
    \caption{More visualization results of our \ourmodel compared to baseline methods. We show the 3D bounding box, text prompt, and two different views.}
    \label{fig:vis_1}
\end{figure*}

\begin{figure*}[!]
   \centering
    \includegraphics[width=\linewidth]{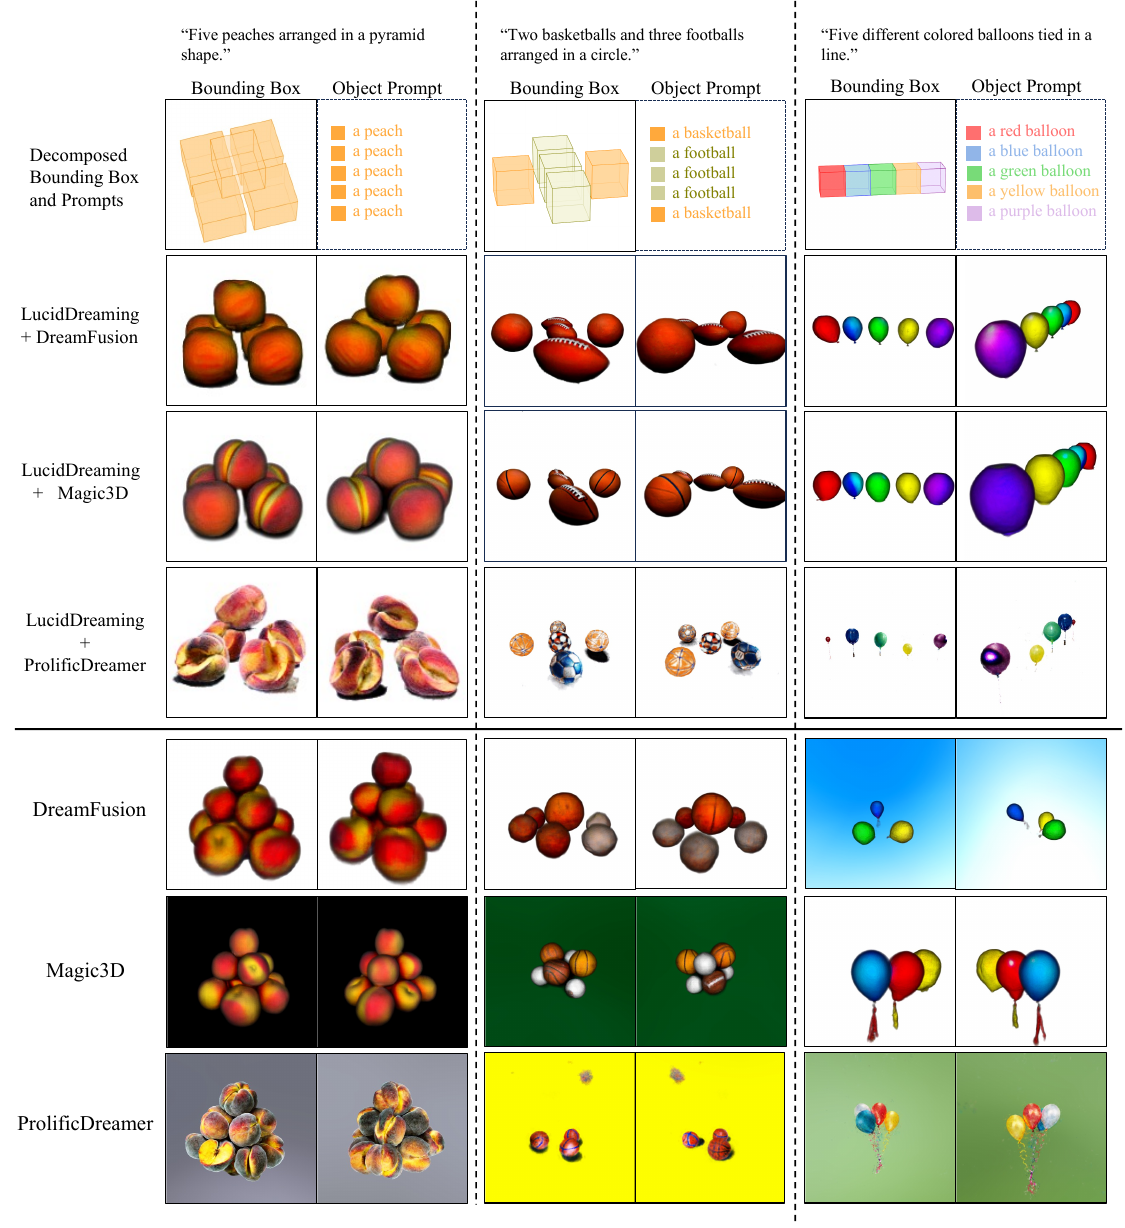}
    \caption{More visualization results of our \ourmodel compared to baseline methods. We show the 3D bounding box, text prompt, and two different views.}
    \label{fig:vis_2}
\end{figure*}

\begin{figure*}[!]
   \centering
    \includegraphics[width=\linewidth]{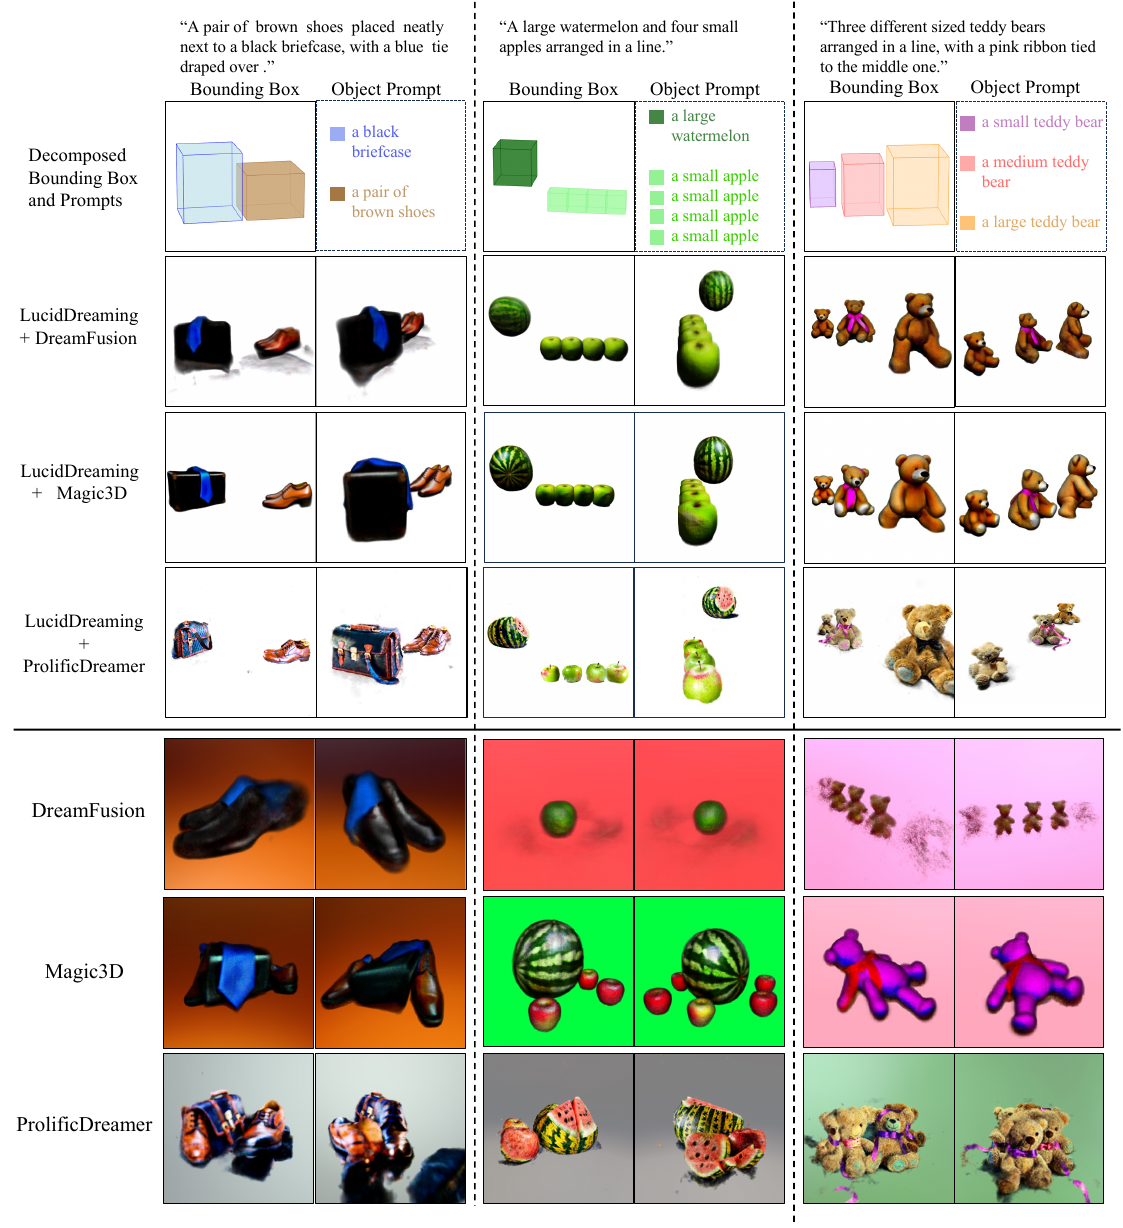}
    \caption{More visualization results of our \ourmodel compared to baseline methods. We show the 3D bounding box, text prompt, and two different views.}
    \label{fig:vis_3}
\end{figure*}

\begin{figure*}[!]
   \centering
    \includegraphics[width=\linewidth]{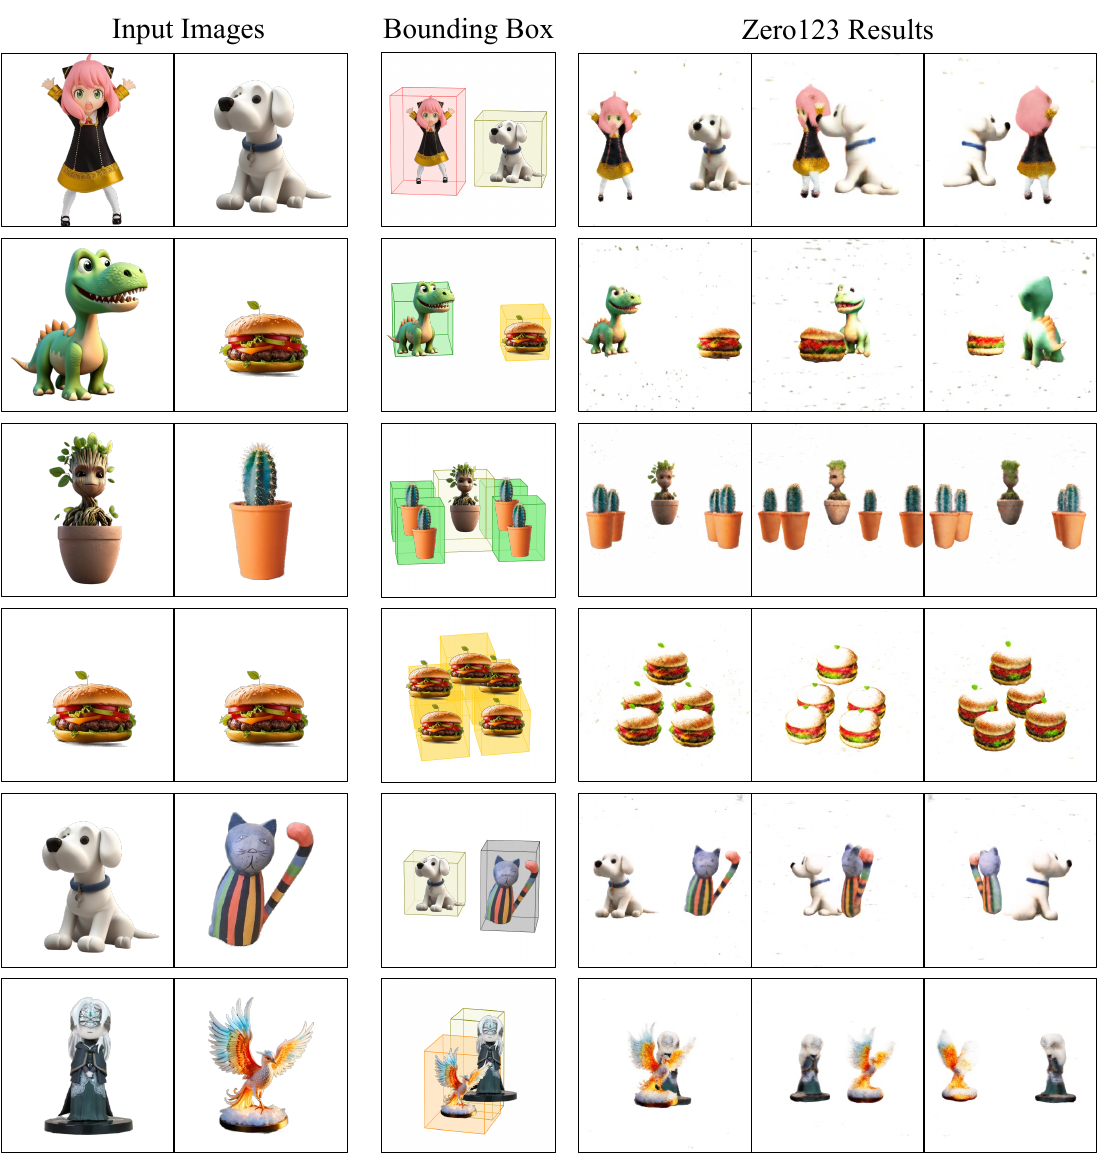}
    \caption{More visualization results of our \ourmodel with \textbf{Zero123}~\cite{liu2023zero} backbone.}
    \label{fig:more_vis_z123}
\end{figure*}

\begin{figure*}[!]
   \centering
    \includegraphics[width=\linewidth]{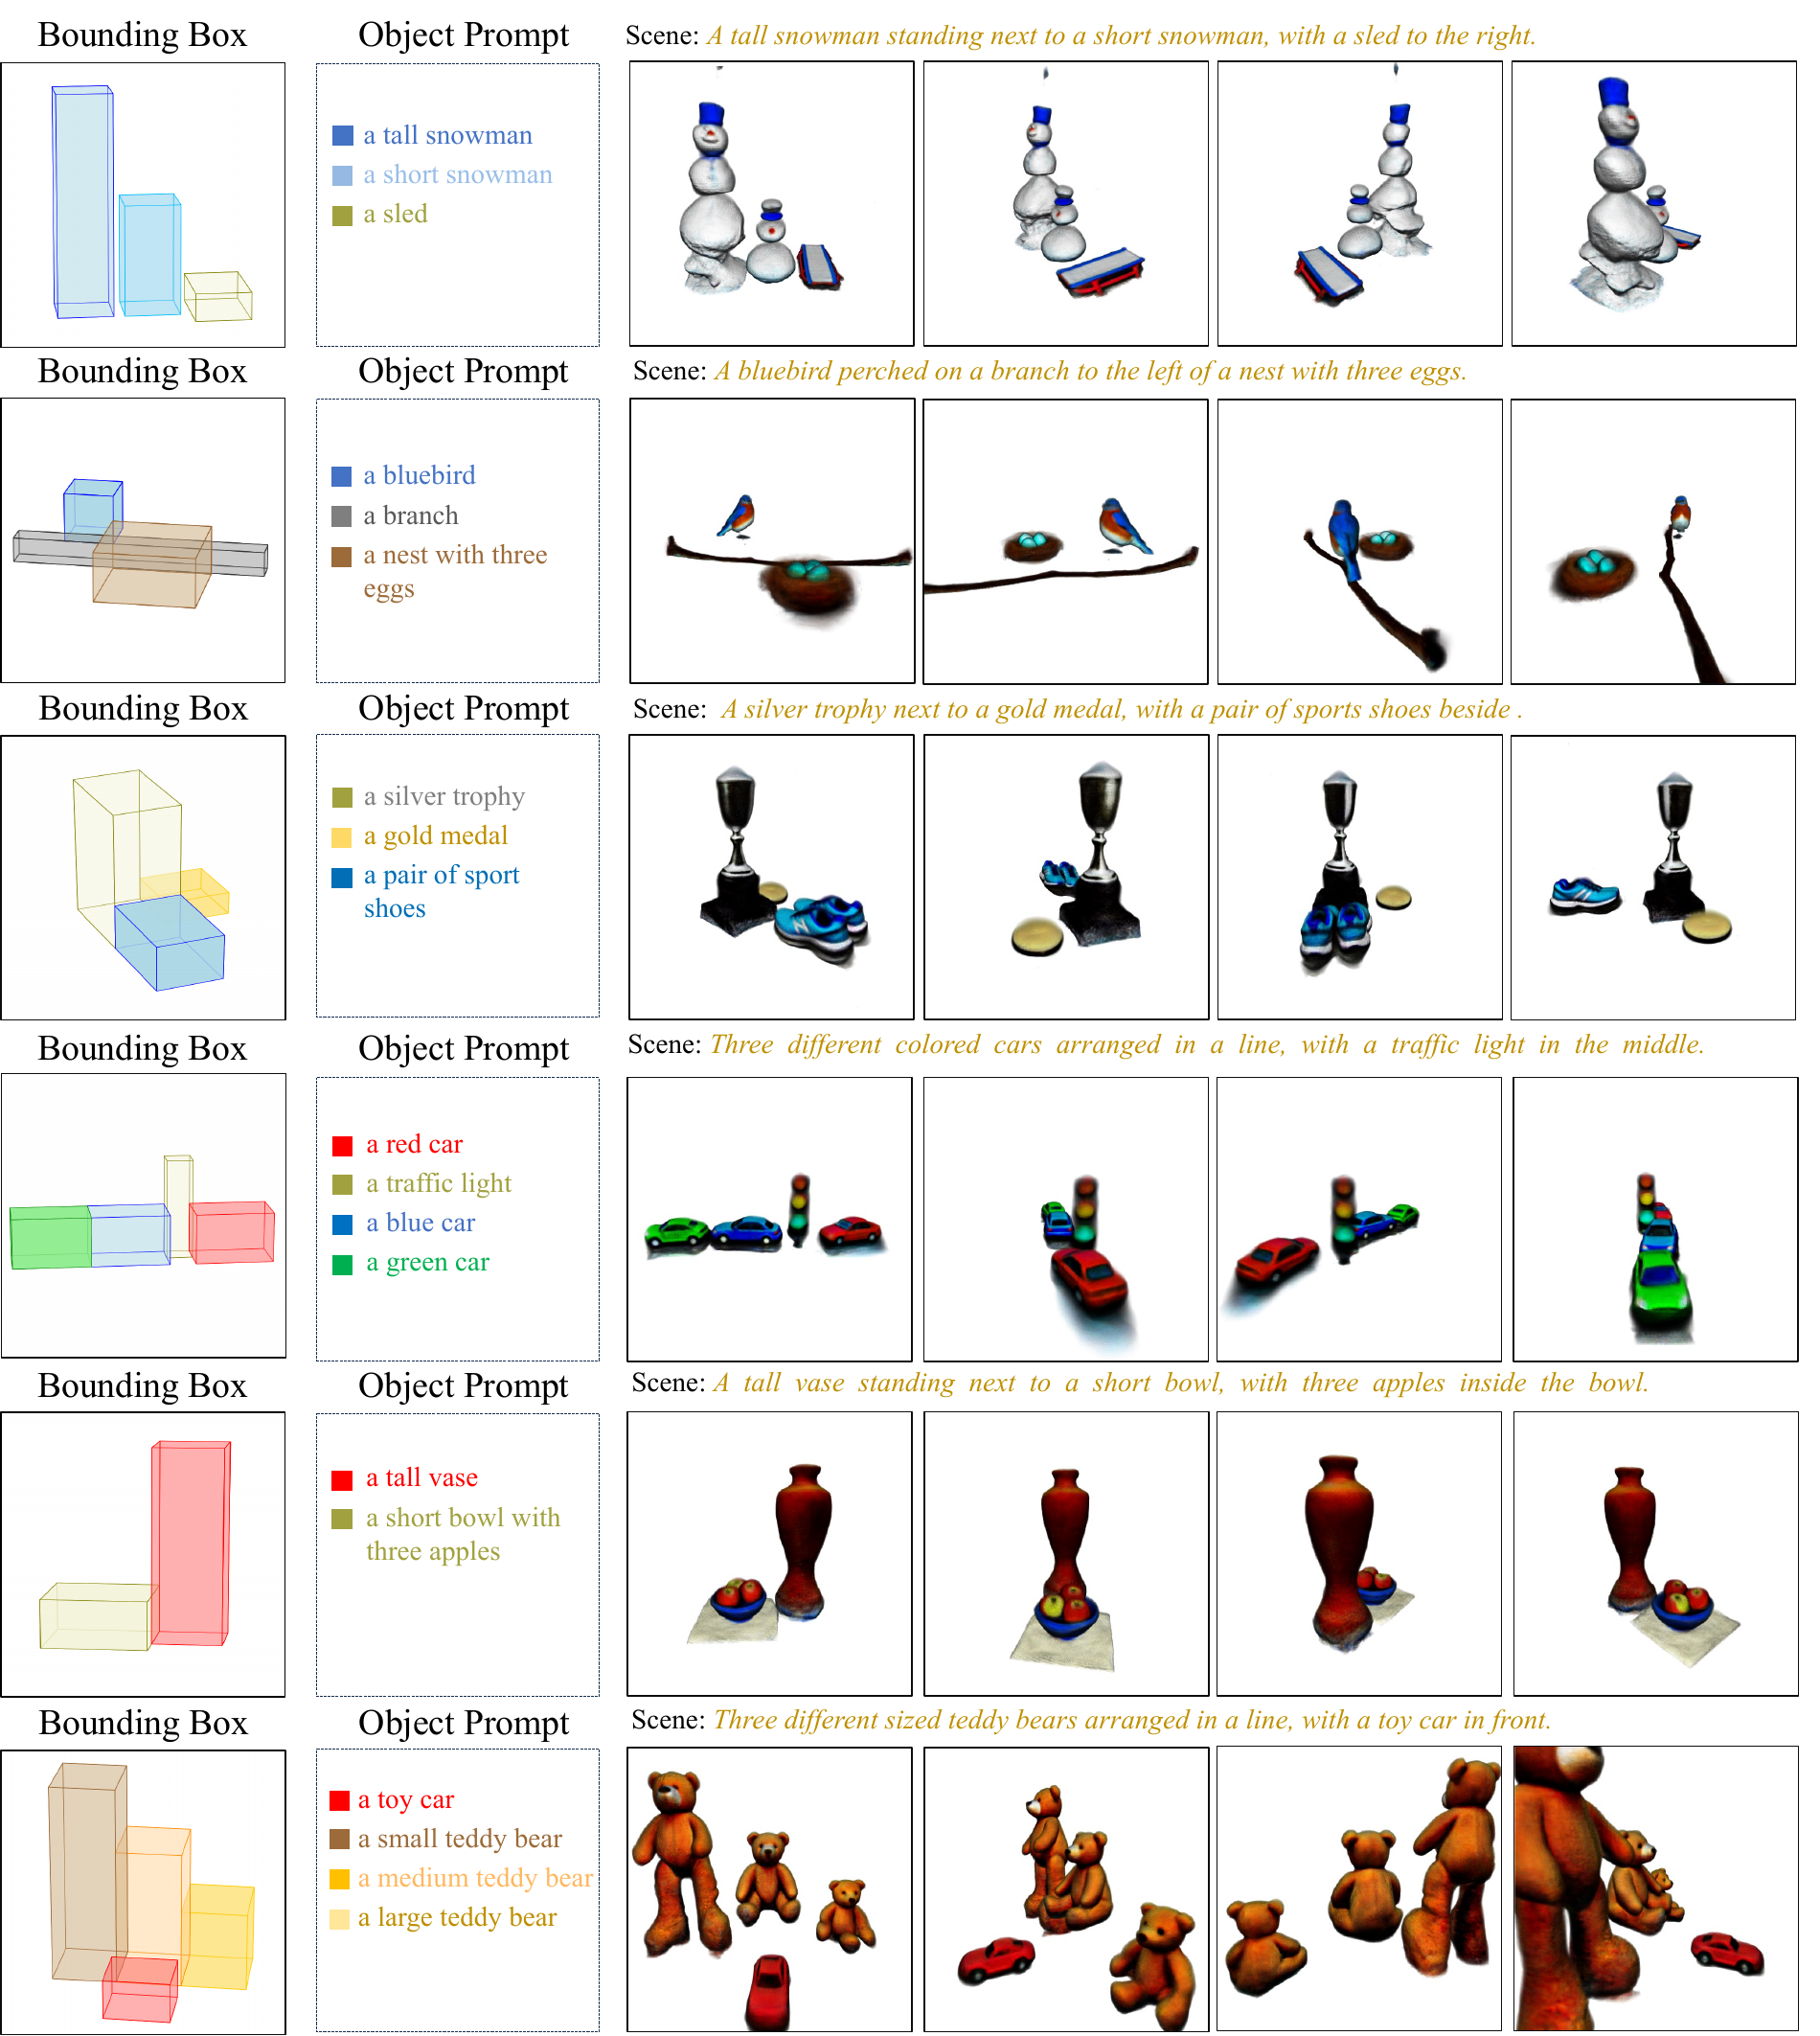}
    \caption{More visualization results of our \ourmodel with \textbf{DreamFusion}~\cite{poole2022dreamfusion} backbone.}
    \label{fig:more_vis_DF}
\end{figure*}

\begin{figure*}[!]
   \centering
    \includegraphics[width=\linewidth]{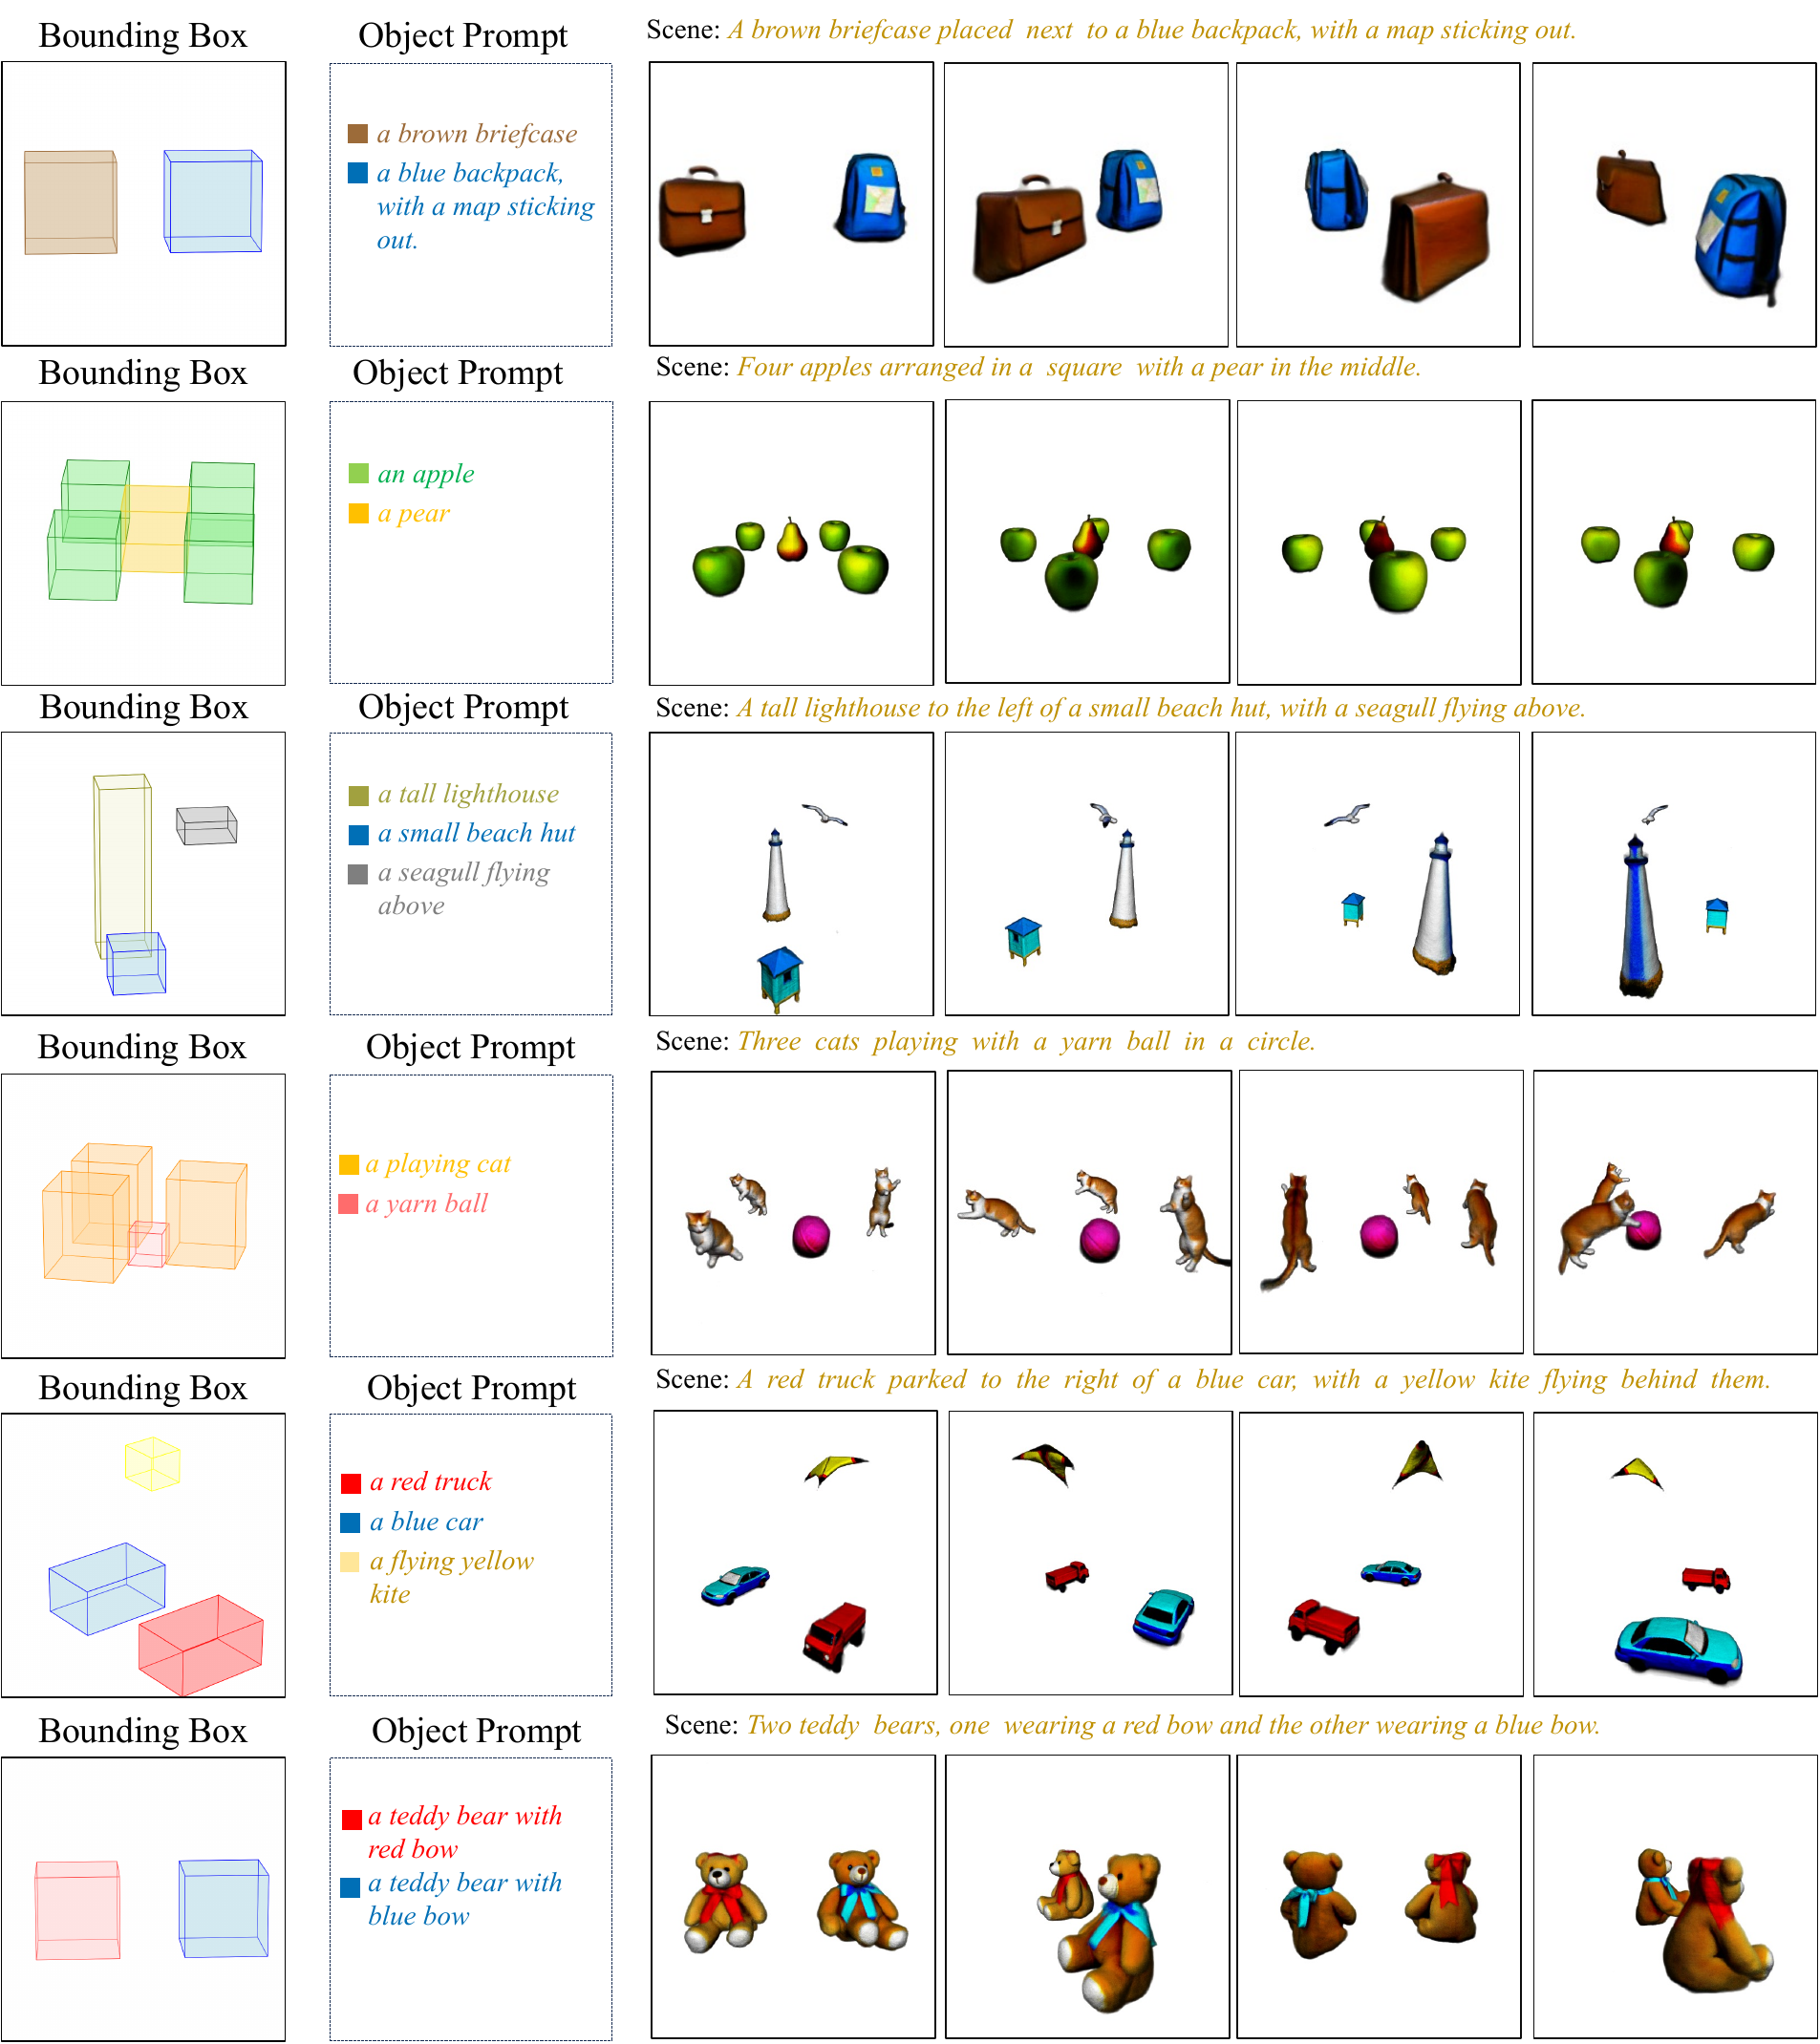}
    \caption{More visualization results of our \ourmodel with \textbf{Magic3D}~\cite{lin2023magic3d} backbone.}
    \label{fig:more_vis_m3d}
\end{figure*}

\begin{figure*}[!]
   \centering
    \includegraphics[width=\linewidth]{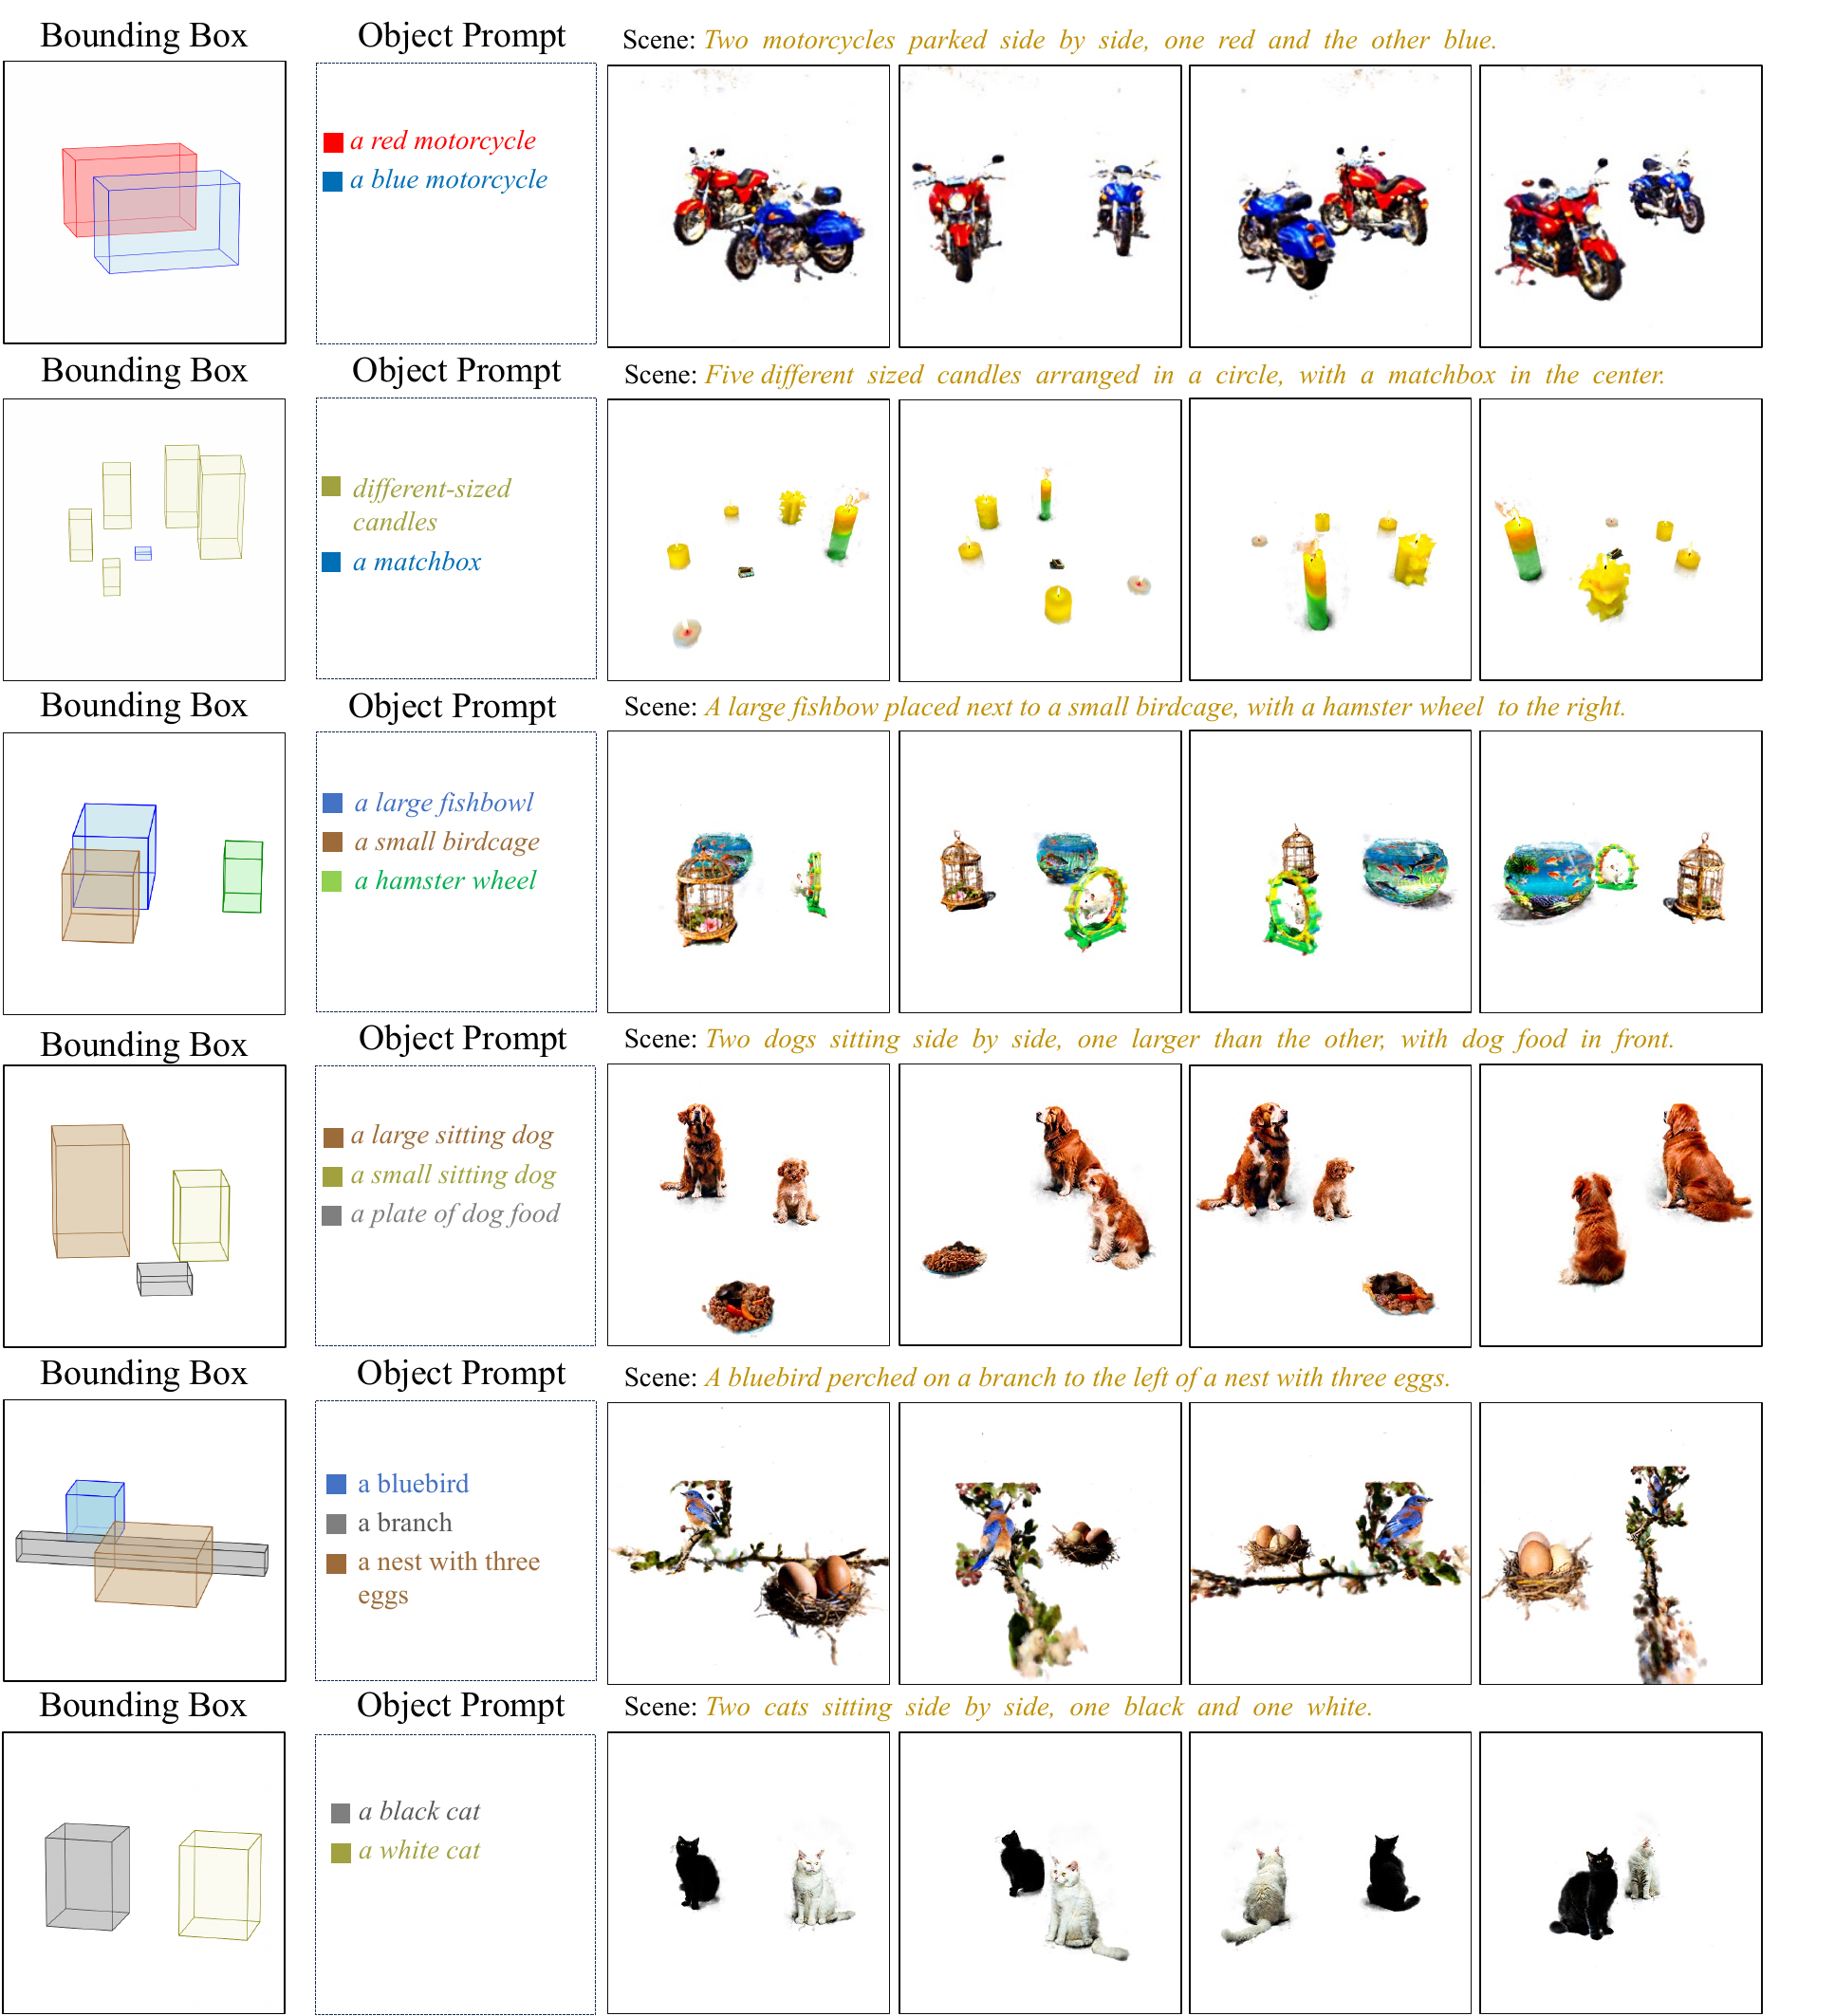}
    \caption{More visualization results of our \ourmodel with \textbf{ProlificDreamer}~\cite{wang2023prolificdreamer} backbone.}
    \label{fig:more_vis_pd}
\end{figure*}

\clearpage
{
    \small
    \bibliographystyle{ieeenat_fullname}
    \bibliography{main}
}
